# Supplementary material for: Relaxed Earth Mover's Distances for Chain- and Tree-connected Spaces and their use as a Loss Function in Deep Learning
Source: arXiv:1611.07573 source file (2016-11-22)
Supplement: Supplementary file 1 [file supplemental_experiments.tex]

%!TEX root = cvpr2017A_supplement.tex
\clearpage
\section{$\EMD$ as pre-training on ImageNet}

\begin{figure}[h]
\centering
\begin{tikzpicture}
\tikzstyle{every node}=[font=\footnotesize]
\begin{axis}[   height=3cm,  width=6cm,
y filter/.code={\pgfmathparse{100*(1-#1)}\pgfmathresult},
scale only axis, ymin=0,ymax=20,xmin=2,xmax=200 ,enlargelimits=false, y label style={at={(axis description cs:-0.075,.5)},anchor=south},  ylabel=Top-1 Accuracy (\%),  x label style={at={(axis description cs:0.5,-0.1)},anchor=north},  xlabel=Epoch, legend cell align=left, legend pos=outer north east, legend style={font=\tiny}]
\addplot+[olive, line width=1pt, mark=none, line join=round] table[x expr=\coordindex+2, y index=1] {results/CE_0_LR005_ErrorRate1.log};
\addplot+[teal,  line width=1pt, mark=none, line join=round] table[x expr=\coordindex+2, y index=1] {results/EMD2_0_ErrorRate1.log};
\addplot+[blue,  line width=1pt, mark=none, line join=round] table[x expr=\coordindex+2, y index=1] {results/SMALL_EMD1.log};
\addplot+[red,   line width=1pt, mark=none, line join=round] table[x expr=\coordindex+2, y index=1] {results/SMALL_EMD_TO_CE1.log};
\legend{$\CE$,$0.5 CE $+$ 0.5 \EMD^2$,$\EMD^2$,$\EMD^2$ until epoch 135 and then $\CE$}
\end{axis}
\end{tikzpicture}
\caption{
Top-1 accuracy on ImageNet using 50K images for training using different loss functions.
The $\CE$ loss strongly favors Top-1 accuracy, therefore it trains fast with regards to this metric.
Conversely, $\EMD^2$ tries to optimize the entire output space resulting in a slower convergence rate.
The combined $0.5 \CE + 0.5 \EMD^2$ shows mixed performance, achieving fast convergence and better accuracy.
However, if we give enough time to let $\EMD^2$ embed the output hierarchy in the network, and then further train the network using the $\CE$ loss we achieve the best results on this metric.
}
\label{fig:pretraining}
\end{figure}

%{\color{red}needs a caption. also, maybe legend to EastOutside?}

In the main paper (Sec. 5.3), we report the results of training on the reduced ImageNet (50K images) dataset using the CrossEntropy~($\CE$) loss alone, the regularized Earth Mover's Distance~($\EMD^2$) loss alone, and an equally weighted combination of the two.
The combined loss $0.5 \CE + 0.5 \EMD^2$ outperforms both individual losses, and also shows fast convergence.

However, as the output space is very large, we think that $\EMD^2$ is not provided the opportunity to learn the output space hierarchy on the model when used in combination with $\CE$.
To test this hypothesis, we perform the following experiment.

We train using the $\EMD^2$ loss until Top-1 accuracy stops improving.
This acts as a pre-training step for the network.
In our experiment this happens at epoch 135.
We then switch the loss function to $\CE$ and employ a very small learning rate (0.001) that only refines the learned parameters of the network.

As $\CE$ strongly favors Top-1 accuracy, it learns on top of the previous network to achieve a Top-1 accuracy of $14.97\%$ (compared to $6.34\%$ for $\CE$, $8.20\%$ for $0.5 \CE + 0.5 \EMD^2$, and $7.66\%$ for $\EMD^2$).
\figref{pretraining} shows the performance for the proposed experiment.
%{\color{red}can you also plot CE + EMD on this?}
